# Supplementary material for: Experimental measurement of respiratory particles dispersed by wind instruments and analysis of the associated risk of infection transmission
Source: arXiv:2205.06481 ancillary file (2022-05-13)
Supplement: Supplementary file 1 [file Supplementary_Information.pdf]

# Supplementary Information: Experimental measurement of respiratory particles dispersed by wind instruments and analysis of the associated risk of infection transmission

Oliver Schlenczek[a], Birte Thiede[a], Laura Turco[a], Katja Stieger[a,b], Jana M. Kosub[c], Rudolf Müller[d], Simone Scheithauer[c], Eberhard Bodenschatz[a,b,e,*], Gholamhossein Bagheri[a,*]

[a]*Max Planck Institute for Dynamics and Self-Organization (MPIDS), Göttingen 37077 , Germany*
[b]*Institute for Dynamics of Complex Systems, University of Göttingen, Göttingen 37077 , Germany*
[c]*Institute of Infection Control and Infectious Diseases, University Medical Center, Göttingen 37075, Germany*
[d]*Institut für Musik und Aerosole, Marsberg, Germany*
[e]*Laboratory of Atomic and Solid State Physics and Sibley School of Mechanical and Aerospace Engineering, Cornell University, Ithaca, NY 14853, USA*

## 1. Supplementary Methods

### 1.1. Subjects

The subjects in our study were either amateur musicians or students of music or graduated musicians. On average, they had 23 years of experience (standard deviation: 19 years) and played their instruments 5 hours per week (range from <1 to 30 hours per week). Their age ranges from 14 to 80 years with a median of 35 years. We had 21 male and 10 female participants. 13 subjects played woodwind instruments only, 17 played brass instruments only, and one subject played both woodwind and brass instruments. 14 of the brass players were male and 4 were female. 8 of the woodwind players were male and 6 were female. 20 types of instruments were examined in our study. One effect the COVID-19 pandemic has introduced into the data is that the subjects did not rehearse and play as often as usual during the time this study was done. Distinction between amateur and professional musicians may have little or no meaning in terms of particle emission, as there is no internationally recognized standard for the playing skills of a musician. Some subjects played only pieces of music, some played a mixture of pieces of music and long single notes, and

*Corresponding author
*Email addresses:* eberhard.bodenschatz@ds.mpg.de (Eberhard Bodenschatz), gholamhossein.bagheri@ds.mpg.de (Gholamhossein Bagheri)

some played just long single notes. This might play a role as the breathing pattern could be different (long single notes need more air). The majority of subject-instrument combinations had 50% or more of the samples in playing a piece of music. Most of the single note experiments were dedicated to examine a possible pitch dependence for the given instrument or to minimize possible leakage from tone holes (the latter for the practice chanter, Great Highland Bagpipes and Scottish Smallpipes). While the majority of these single notes led to lower particle emission than the piece of music played, or approximately the same range, some special notes led to more than an order of magnitude higher emission (for example overblowing the reed of the clarinets). These notes, however, contribute to less than 20% of the samples, so they did not influence the mean particle emission by much. As we found the emission from playing long single notes to be mostly comparable or below the emission from playing a piece of music, we included them for the calculation of the mean emission, knowing that this might lead to an underestimation of the typical emitted particle number and volume concentration for some subjects and instruments.

### *1.2. Particle losses within the aerosol sampling setup*

Even though the measured particle number and volume concentrations in this work are often higher than the highest values found in other studies for the same instruments, we know that there is a non-negligible loss of particles on the inner walls of the tubing and also on the meshes inside the two diffusion dryers. In a comparison measurement with a very high particle background concentration of dry dolomite dust (number concentration $\approx 250\,\mathrm{cm}^{-3}$), we found a loss rate of 19% from the two diffusion dryers across the full size spectrum. The setup was built in a way that the tube lengths and the bend radii were the same between the section with the dryers and the section without dryers. This loss rate did not change by much for lower or higher concentration and it was also nearly independent of particle diameter. As we did not observe a substantially lower particle concentration in the measurements with the standard setup compared to direct OPS measurements, we can conclude that dilution of exhaled air in front of the OPS inlet nozzle has about the same effect on the measured concentration as the losses in tubing and dryers. The losses need to be considered when discussing the infection risk. To get an idea of the particle loss percentage for different particle sizes, the Particle Loss Calculator (von der Weiden et al., 2009) was applied to different measurement scenarios during this study. The four scenarios of interest are shown in Fig. 1. Higher volumetric flow rates were associated with lower losses of particles around 5 µm diameter. However, even the plain inlet nozzle of the OPS introduces some losses in the larger size bins (about 25% loss for 9 µm). In case of the standard setup with both diffusion dryers, tubing and collection funnel, we find loss rates between 40% and 75% for particles of 5 µm diameter. For 8 µm and larger, we expect a loss rate of 90% or more, with already between 50% and 90% particle loss in the section from the collection funnel to the first diffusion dryer. These numbers show that anything above 5 µm particle diameter at the funnel rim is most likely lost within the setup, and our analysis should focus on the particulate matter

Table 1: Overview of instruments and subjects. Shown are instrument ((P) for piston valves, (R) for rotary valves) played, number of (unique) experiments (one specific title or note played with funnel on bell end), number of samples, experiments with mask, usage of additional particle spectrometers, and percentage of single long note samples. The asterisk highlights a flute with a B attachment.

| No. | Instrument | Exp. | Samples | Mask | SMPS | APS | % notes |
|---|---|---|---|---|---|---|---|
| 1 | Trumpet (P) | 5 | 16 | Yes | Yes | Yes | 0 |
| 2 | Soprano sax | 2 | 4 | No | Yes | Yes | 0 |
| 2 | Tenor sax | 2 | 5 | No | Yes | Yes | 0 |
| 3 | Clarinet | 2 | 3 | Yes | Yes | Yes | 33 |
| 4 | Trumpet (R) | 2 | 2 | Yes | Yes | Yes | 50 |
| 5 | Alto sax | 2 | 2 | Yes | Yes | Yes | 50 |
| 6 | Flute* | 2 | 3 | Yes | Yes | Yes | 33 |
| 7 | Trumpet (P) | 4 | 10 | Yes | No | No | 0 |
| 7 | Tenor sax | 3 | 3 | Yes | Yes | No | 0 |
| 8 | Flute | 2 | 3 | Yes | Yes | No | 33 |
| 8 | Alto recorder | 3 | 5 | Yes | Yes | No | 20 |
| 9 | Trumpet (R) | 1 | 2 | Yes | Yes | No | 0 |
| 10 | Trombone | 1 | 2 | Yes | Yes | No | 0 |
| 11 | Clarinet | 2 | 3 | Yes | Yes | No | 33 |
| 12 | Trombone | 1 | 1 | Yes | Yes | No | 0 |
| 13 | G. H. Bagpipes | 1 | 3 | Yes | No | No | 100 |
| 13 | Sc. Smallpipes | 1 | 8 | Yes | No | No | 100 |
| 13 | Practice chanter | 1 | 6 | Yes | No | No | 100 |
| 14 | Trumpet (P) | 1 | 3 | No | No | No | 0 |
| 15 | Trombone | 2 | 3 | Yes | No | No | 0 |
| 16 | F tuba (R) | 3 | 8 | Yes | No | No | 0 |
| 17 | Double horn (R) | 2 | 15 | Yes | No | No | 0 |
| 17 | Trombone | 2 | 15 | Yes | No | No | 0 |
| 18 | Tuba (R) | 3 | 11 | Yes | No | No | 0 |
| 19 | Trombone | 1 | 5 | Yes | No | No | 0 |
| 20 | Tenorhorn (R) | 1 | 5 | Yes | No | No | 0 |
| 21 | Tuba (R) | 2 | 7 | Yes | No | No | 0 |
| 22 | Tenorhorn (R) | 1 | 5 | Yes | No | No | 0 |
| 23 | Trombone | 1 | 4 | Yes | No | No | 0 |
| 24 | Clarinet | 7 | 15 | Yes | No | No | 43 |
| 24 | Alto sax | 2 | 4 | Yes | No | No | 100 |
| 24 | Tenor sax | 2 | 4 | Yes | No | No | 100 |
| 25 | Clarinet | 7 | 10 | Yes | No | No | 60 |
| 26 | Clarinet | 6 | 8 | Yes | No | No | 50 |
| 27 | Soprano sax | 6 | 12 | Yes | No | No | 58 |
| 28 | Piccolo | 6 | 12 | Yes | No | No | 58 |
| 28 | Flute | 5 | 9 | Yes | No | No | 44 |
| 29 | Fife | 6 | 12 | Yes | No | No | 42 |
| 30 | Kuhlo horn (R) | 7 | 10 | Yes | No | No | 60 |
| 30 | Picc. trumpet (P) | 3 | 4 | Yes | No | No | 75 |
| 31 | Hunting horn | 3 | 16 | Yes | Yes | No | 100 |
| 31 | Trumpet (P) | 2 | 32 | Yes | Yes | No | 100 |

smaller than 5 µm (PM5) fraction. Taking the results from the intercomparison in Subsection 2.2 into account, it is actually PM5 dry for all wind instruments data, and not PM5 at exhalation.

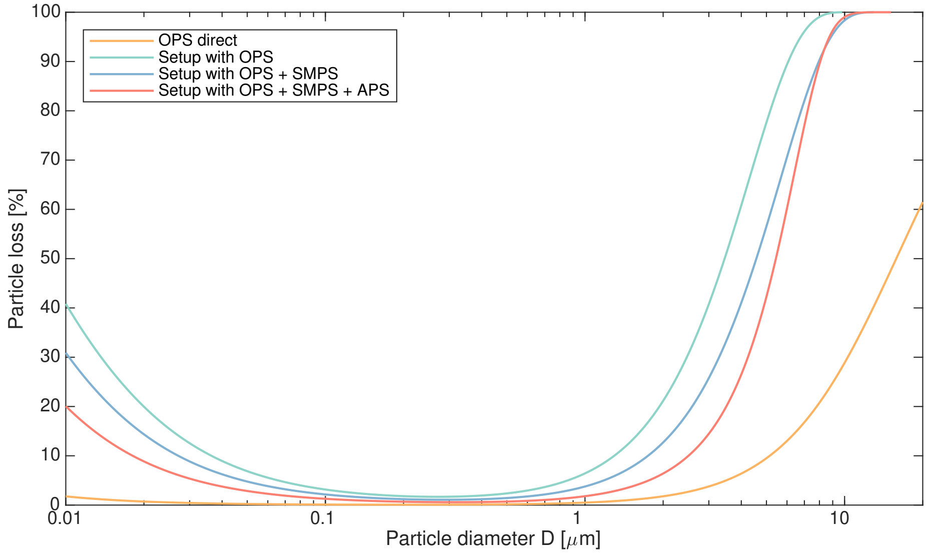


Figure 1: Calculated particle loss (in %) as a function of particle diameter. The calculations are based on length, diameter, orientation and curvature angle of the tubing, sample flow rate, and velocity of the particle-laden air and were done with the Particle Loss Calculator (von der Weiden et al., 2009). The volumetric flow rates were $1\,\mathrm{L\,min^{-1}}$ for "OPS direct" and "Setup with OPS", $1.75\,\mathrm{L\,min^{-1}}$ for "Setup with OPS + SMPS", and $6.75\,\mathrm{L\,min^{-1}}$ for "Setup with OPS + SMPS + APS".

### *1.3. Working principle of wind instruments*

The main physics of wind instruments are quite simple and consist of two parts: the generator of the tone and the resonator. The generator can be a sharp edge (e.g. flute, recorder or pipe organ), a single reed (e.g. clarinet or saxophone), a double reed (e.g. oboe, bassoon and most bagpipes) or the vibrating lips of the player (all brass instruments). The tube of the instrument is the resonator and its function is to amplify the tone that comes from the generator, and to shape the harmonics spectrum. It does so by generating a standing sound wave, so the tube length and the medium (in most cases air) determine the frequency of resonance. Other effects like the gradual widening of the tube towards the bell end are not discussed here. By itself, the instrument is limited to the natural harmonics series. There are two ways to allow chromatic playing. One is to shorten the resonator length by placing tone holes between the mouthpiece and the bell end, which is done for woodwind instruments. Another possibility is to increase the resonator length by using a slide (common for most trombones) or by attaching additional tubes to the instrument which can be

engaged or disengaged by the use of piston or rotary valves (most modern brass instruments). Due to the large number of openings (e.g. clarinets typically have 22 holes or more), the mechanics and aerodynamics of some woodwind instruments are very complicated and require a detailed analysis to quantify the net particle emission. Instruments like the clarinet and the oboe are played in different registers. To change from the low to the high register, the player opens a so-called register key. Woodwind instruments with a cylindrical bore (for example a clarinet) sound at triple the original frequency when overblowing while instruments with a conical bore (like an oboe) sound at the double of the original frequency. There are some less common instruments like the ophicleide or the cornett, which are part of the brass family but have tone holes. Here, we will focus on brass instruments without tone holes. Commonly used brass instruments have the most simple aerodynamics of all wind instruments as they have one single inlet (the mouthpiece) and one single outlet (the bell end). The resistance experienced when playing a wind instrument is lowest for playing just the mouthpiece (brass, single-reed and double-reed woodwind instruments). With the resonator connected, the playing resistance increases. The higher resistance might have an influence on the particle emission which has not been quantified so far. There are instruments with different meanings in English and German, for example the tenorhorn. In Germany, a tenorhorn is a low brass instrument with the same fundamental pitch as a tenor trombone, which is equipped with rotary valves. In some countries, a tenor horn is a brass instrument with piston valves and tuned in E-flat, which sounds a perfect fourth higher than a tenorhorn. Other differences are for example that most tubas played in Germany have rotary valves, and many trumpet players in German symphonic orchestras tend to prefer playing trumpets with rotary valves. A summary of the different instrument types is shown in Table 2. The hunting horn played in this study does not have valves and is therefore limited to the natural harmonics series.

Table 2: Properties of different wind instrument types. Mixed tube bore means the tube is mostly cylindrical, except for the piece close to the bell end. For the bagpipes, the shape of the chanter is mentioned. The drones are usually straight single-reed in windcap.

| Instrument type | Category | Shape | Tube bore |
|---|---|---|---|
| Piccolo | Edge-blown | Straight | Cylindrical |
| Fife | Edge-blown | Straight | Cylindrical |
| Flute | Edge-blown | Straight | Cylindrical |
| Alto recorder | Edge-blown | Straight | Cylindrical |
| Clarinet | Exposed single-reed | Straight | Cylindrical |
| Soprano sax | Exposed single-reed | Straight | Conical |
| Alto sax | Exposed single-reed | Curved | Conical |
| Tenor sax | Exposed single-reed | Curved | Conical |
| Practice chanter | Double-reed in windcap | Straight | Conical |
| Great Highland Bagpipes | Double-reed in windcap | Straight | Conical |
| Scottish Smallpipes | Double-reed in windcap | Straight | Cylindrical |
| Piccolo trumpet | Brass | Curved | Mixed |
| Trumpet | Brass | Curved | Mixed |
| Kuhlo horn | Brass | Curved | Conical |
| Hunting horn | Brass | Curved | Conical |
| Tenor trombone | Brass | Curved | Mixed |
| Tenorhorn | Brass | Curved | Conical |
| Double horn | Brass | Curved | Mixed |
| F tuba | Brass | Curved | Conical |
| Bb tuba | Brass | Curved | Conical |

## 2. Supplementary Results

### *2.1. Particle spectrometer intercomparison*

An intercomparison between an APS and an OPS was done by emitting the exhaled air directly into the sample inlet of both instruments in subsequent experiments of the same kind. No funnel or tubing was used here. This intercomparison was done for playing the trumpet over a period of 1 min. Fig. 2 shows the size distribution measured while playing the trumpet, assuming that the particles are spherical. There is a reasonable agreement between the two devices with the OPS having better sensitivity in the small diameters. Also, we see a reduction in detectability in the APS data for particles larger than 4 µm, which is consistent with the reduced counting efficiency of the APS for larger sizes mentioned in Pöhlker et al. (2021). In particular for the wind instruments we found the size channels from 0.3 to 0.5 µm to be extremely important for measuring reasonable number concentrations (for most of the examined wind instruments, about 80% of the total number concentration $N$ was found below 0.5 µm).

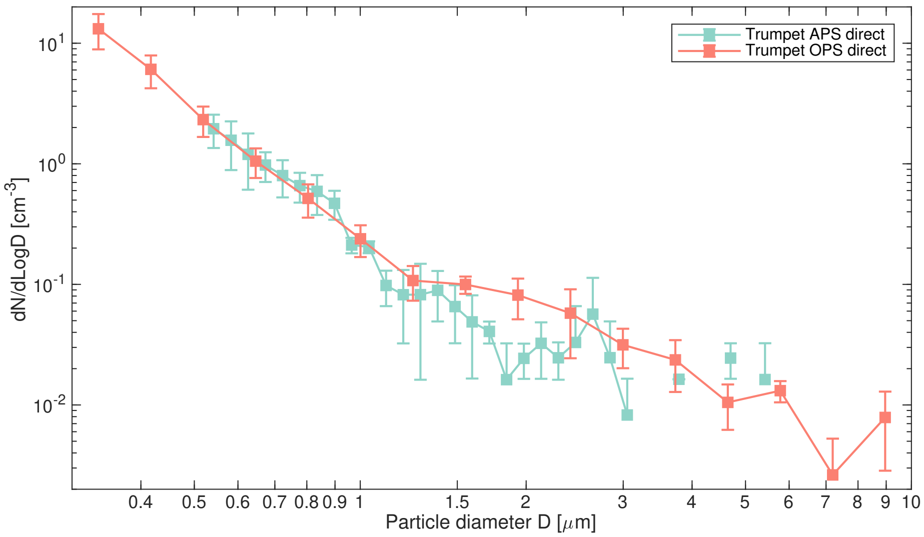


Figure 2: Particle size distributions measured directly at the APS inlet nozzle (green) and the OPS inlet nozzle respectively (red) for playing the trumpet. Shown are the median size distribution (squares) and standard error (errorbars).

### *2.2. Shrinkage factor for dry versus exhaled particle diameter*

For a relatively short measurement duration (less than 5 min of playing without interruption), the wind instruments seem to act like a dryer, as the measured size distributions for direct OPS measurements and measurements via funnel and dryers overlap for two subjects who played the trumpet (Fig. 3) and the

clarinet respectively (Fig. 4). About 5 min is a typical duration of a piece of light music played at a fair or a Schützenfest, which is usually followed by a short break. In score for symphonic orchestra, there are numerous pieces for one voice which are longer than 5 min.

The fact that the measured concentration with the funnel was higher than with the direct measurement can be attributed to less dilution of the exhaled air with the funnel compared to the wide opening of the instrument bell and the tiny inlet of the OPS, and much more space for ambient air to be entrained in the exhale jet. When comparing the particle size distributions sampled with the funnel from a tuba, we do not see a significant difference between the experiments with diffusion dryers and without diffusion dryers (and shorter tube length) other than a higher loss rate with the standard setup (OPS + SMPS + both Grimm dryers).

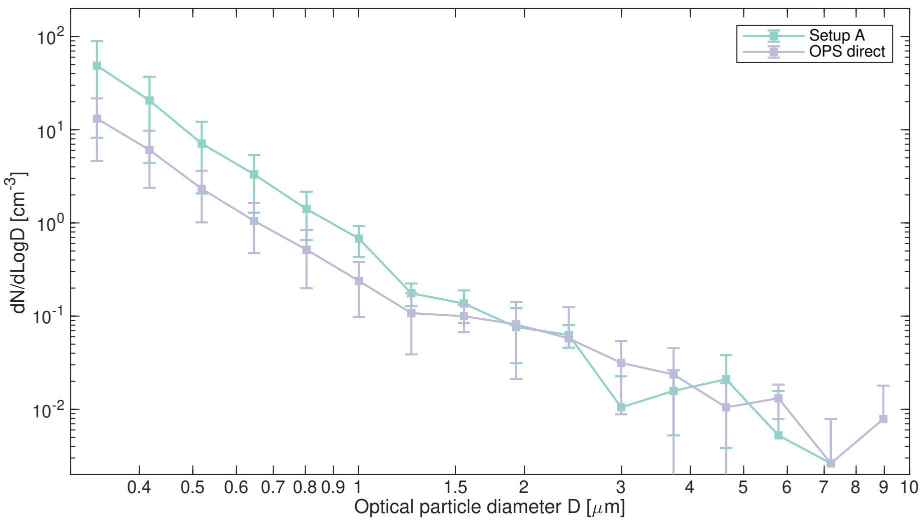


Figure 3: Size distributions for playing a trumpet, measured either with the standard setup (100 mm funnel) or directly (OPS direct). The same pieces of music were used in two experiments of two samples each. Shown are the size distributions for the measured diameter, with $D_0/D_{dry} = 1$.

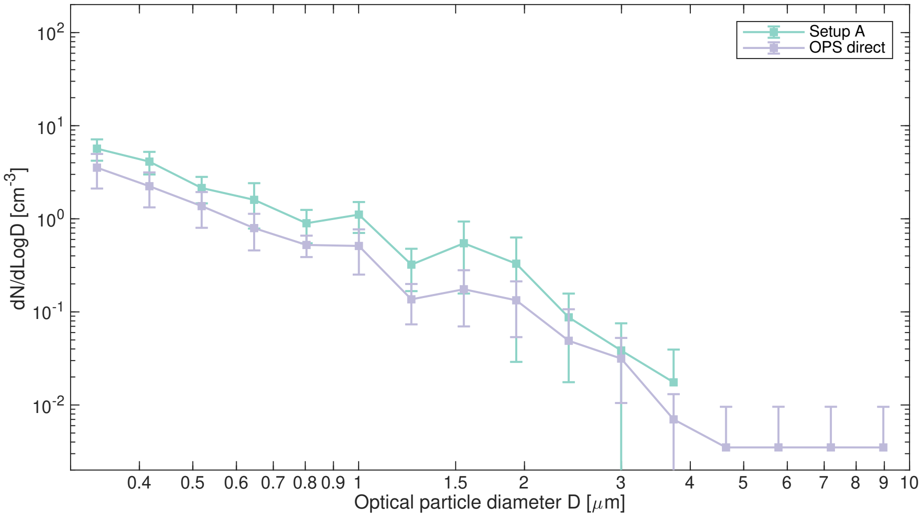


Figure 4: As in Fig. 3 for playing a clarinet.

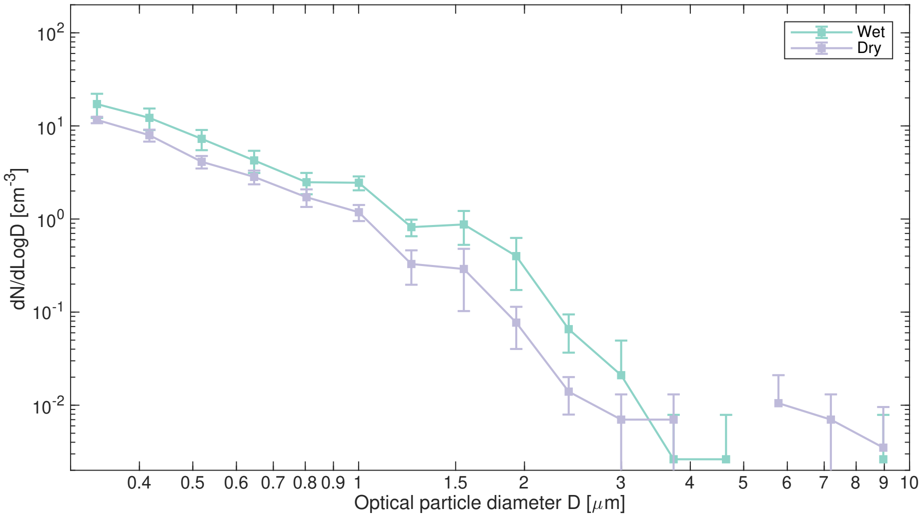


Figure 5: As in Fig. 3 for playing a F tuba.

### 2.3. Sampling time

The measurement time plays a big role in the assessment of the emitted $N$ under conditions close to real concert or rehearsal situations (equilibrium conditions). As the air in the instrument is free of particles in the beginning (there was a null test done before the actual measurement, which was flushing the instrument with particle-free compressed air), it will take some time of playing to measure the undiluted exhaled particle concentration. This time depends on the instrument. For a B-flat tuba, the delay was the longest. The playing was started 30 s before the end of Sample 3 (each minute in Fig. 6 is the end point of each sample), and it took another full sample until equilibrium conditions were reached. There is some variability visible in the data, in particular in the small sizes, but overall the emitted $N$ during each piece of music was quite consistent. An important question to ask when comparing results with other studies is if equilibrium conditions for particle emission from the instruments were reached.

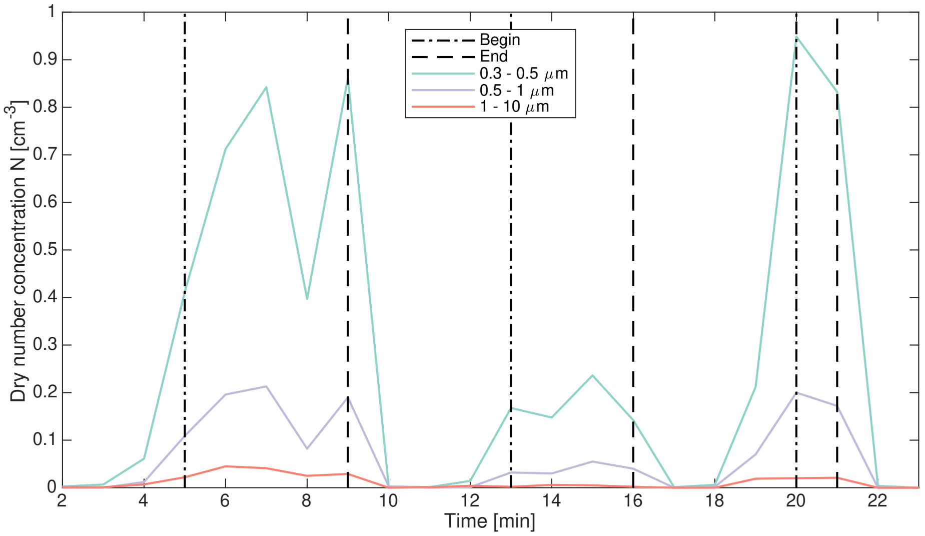


Figure 6: Time series of a subject playing three different titles on a B-flat tuba. Begin (dash-dotted lines) and end (dashed lines) of the measurement range are marked and shown together with the particle number concentration for the sizes below 0.5 µm (green), between 0.5 and 1 µm (purple), and larger than 1 µm (red). The rest between the experiments was 2 minutes.

### 2.4. Possible disturbances of particle measurements on wind instruments

There are several effects which could lead to systematic errors when examining the particle emission of wind instruments. One of them is the possible presence of particles in the instruments before playing. To minimize the effect of measuring dust or dry residues released from the inner walls of the instruments, it is recommended to flush the instrument with particle-free air before starting the measurement. If this is not possible, the instrument should be

played for several minutes before taking the first sample. The condensing water in the instrument will help to capture dust and keep it from being released at the bell end.

Another effect that was found to have a significant impact on the measured particle concentration is the usage of lubricants such as valve oil in brass instruments. For a synthetic valve oil, we measured particle number concentrations that were by a factor of 6-7 higher, and volume concentrations were by a factor of 26-44 higher compared to the emission before using valve oil. For a vegetable-based valve oil, we found an increase in number concentration by a factor of 4, and an increase in volume concentration by a factor of 1.5. There are several possible effects that could explain the higher measured number and volume concentration after oiling the valves. One effect is most likely the hydrophobic nature of the oil, which could suppress wet deposition inside the instrument. In addition, small interstitial aerosol particles could grow via oil vapor deposition and, due to the lower vapor pressure of the oil compared to water, pass the diffusion dryers without much evaporation to be finally detected by the OPS.

### *2.5. Particle leakage*

With the setups B and C as described in Fig. 1 in Materials and Methods of the main paper, we investigated the role of leakage at the tone holes and also around mouth and nose during the play. For the leakage around mouth and nose, we have data from two trumpet players, two trombone players, two soprano sax players, one piccolo player, one fife player, and three flutists. The emitted particle size distribution measured in front of mouth and nose was compared with the average particle size distribution for normal breathing based on the data in Bagheri et al. (2021a) for the six instruments mentioned. Fig. 7 shows the size distributions. Apart from the trumpet data, where a higher mean concentration is found between 4 and 20 µm exhaled diameter, all other size distributions measured in front of mouth and nose are very consistent with the mean fitted size distribution for normal breathing. Due to that, we assume breathing to be responsible for most of the emission measured in front of mouth and nose. This needs to be taken into account when calculating the risk of SARS-CoV-2 transmission if the infectious plays a wind instrument and does not wear a face mask.

In addition to the leakage in front of mouth and nose, we also examined leakage from the tone holes in a series of experiments where one subject played a clarinet, an alto sax and a tenor sax. For each experiment, the same note was played and the size distributions measured with setup A are compared to setup C in Fig. 1 in Materials and methods of the main paper. In all experiments, the bell end was open and the tube end (for measurement of leakage at a tone hole) was approximately 1 cm away from the tone hole to avoid systematic errors due to under-pressure. Fig. 8 shows the size distributions measured at the bell end with Setup A in comparison to the size distributions measured at the tone holes with setup C. In case of the tenor sax and the clarinet, we see very similar size distributions from the bell end and from the tone holes. Only in case of the alto sax, the emission at the bell end was visibly higher

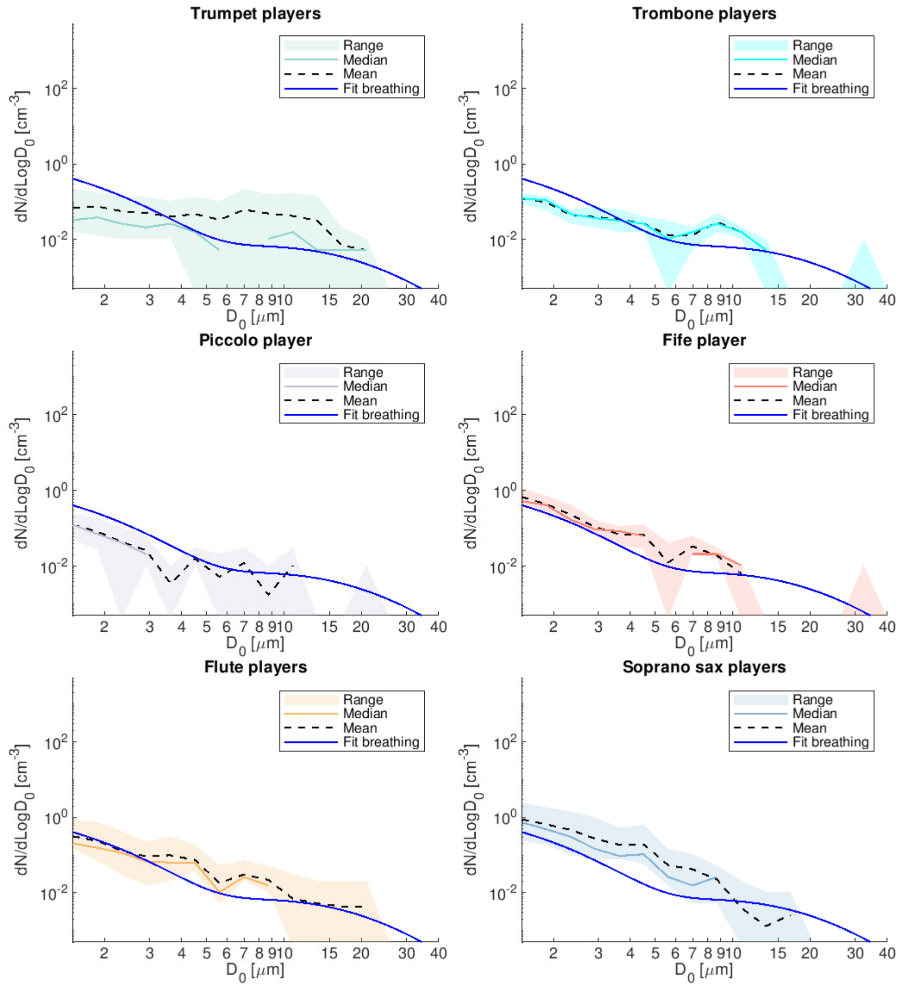


Figure 7: Size distributions measured via Setup B (funnel in front of mouth and nose) for trumpet (top left), trombone (top right), piccolo (middle left), fife (middle right), flute (bottom left), and soprano sax (bottom right) in comparison with normal breathing from multi-modal log-normal fit in Bagheri et al. (2021b) (solid blue line). The shaded area represents the range from 25th percentile to maximum.

than at the tone holes. Even with this setup, which does not take all the tone holes into account simultaneously, we clearly see that a substantial part of the emitted particles escape from the tone holes. This strengthens the argument of Firle et al. (2021) that masks at the bell end are not sufficient to reduce particle emission from woodwind instruments. And this finding contradicts the conclusion by Stockman et al. (2021) that surgical masks are effective for woodwind instruments such as clarinets. Finally, we need to assume that the leakage from the tone holes can be about the same as the emission measured at the bell end.

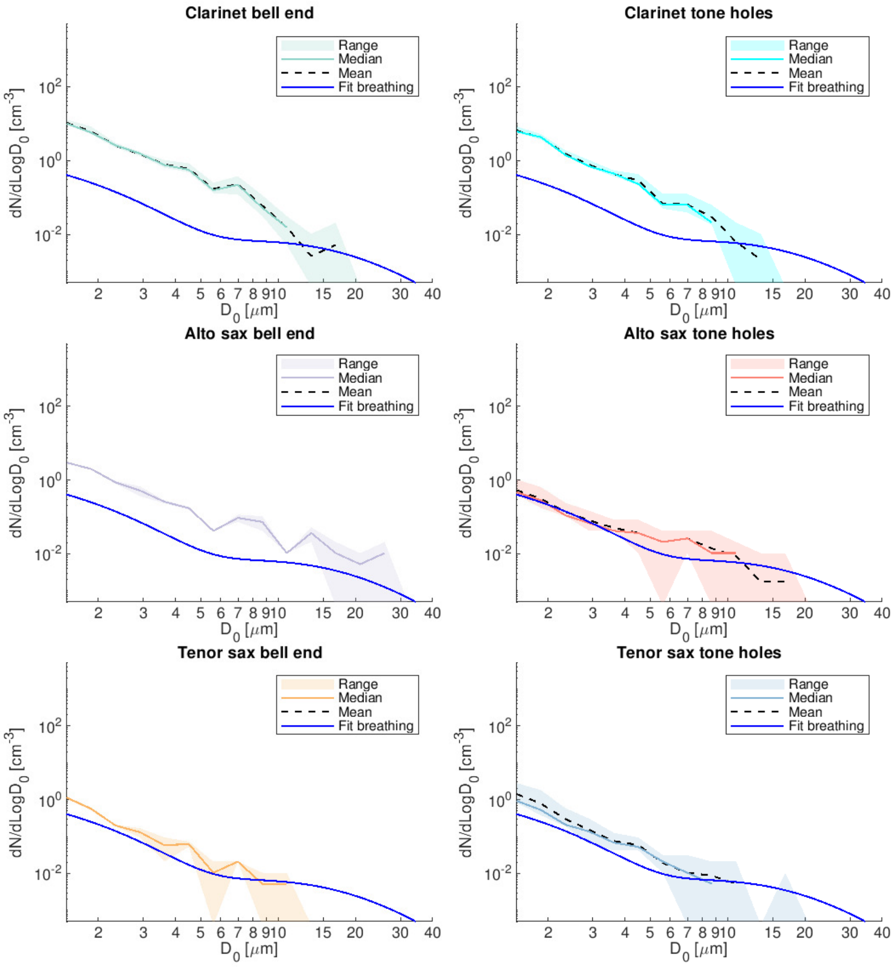


Figure 8: Comparison of size distributions measured via Setup A at instrument bell end (left) and size distributions measured via Setup C at the tone holes (right). Shown are data for a clarinet (top), alto sax (middle) and tenor sax (bottom row). The shaded area represents the range from 25th percentile to maximum, the solid blue line is the multi-modal log-normal fit for normal breathing in Bagheri et al. (2021a).

## 2.6. Comparison with previous studies

An overview of the recently published data on particle emission by different wind instruments is given in Table 3. We restricted our measured particle concentration to the range that was also possible to measure with an APS. As the number of particles >10 µm was very low, we think that the restricted OPS range and the native APS range are comparable in terms of particle number concentration. As described in He et al. (2021) and Stockman et al. (2021), their APS-based measurements used a conductive silicone tube with 0.15 m length (Stockman et al., 2021) at about 15 cm distance from the instrument bell, and a conductive silicone tube of 0.5 m length with three funnels of different size, one of them selected to match the bell size of the particular instrument (He et al., 2021). The setup used in this study had a 3.5 m long conductive PTFE tube of 6 mm inner diameter with two diffusion dryers in between, yielding a total tube length of 4.2 m. Thus, we expect higher loss rates for particles larger than 4 µm compared to the setups used by He et al. (2021) and Stockman et al. (2021) as visible in Figures 8 and 9 of SI. As already pointed out earlier in this paper, the majority of emitted particle number concentration was found in the sub-micron range, so the differences between the studies compared in Table 3 should not be due to different particle loss rates. Moreover, we know from our intercomparison with OPS direct measurements that the particle size distributions measured at the bell end of wind instruments is the dry particle diameter (see Subsection 2.3 and Figures 7, 8 and 9 of SI).

In comparison with the results published by He et al. (2021) and Stockman et al. (2021), we find our values of particle number concentration $N$ mostly in the same range. The fact that the measured number concentration for the flute by Stockman et al. (2021) was below our minimum is most likely due to the higher background particle concentration in their study (they mention a background $N$ between 0.03 and 0.1 $cm^{-3}$). We assume that He et al. (2021) measured a B-flat tuba in their study, and we speculate that the low values for $N$ might be due to the shorter duration of play. We examined longer duration of playing the tuba as shown in the example of Fig. 11 (Subsection 2.5.) in SI. All other disparities between our study and the results published by He et al. (2021) and Stockman et al. (2021) are explainable by between-subject variability, and possibly also the selection of the music played. The between-subject variability needs also to be taken into account when discussing our results from instruments played by a single subject.

| Instrument type | He et al. (2021): $N_{0.5-20}$ [$\mathrm{cm}^{-3}$] | Stockman et al. (2021): $N_{0.5-20}$ [$\mathrm{cm}^{-3}$] | This work: $N_{0.5-10}$ [$\mathrm{cm}^{-3}$] |
|---|---|---|---|
| Bass clarinet | 0.06 | | |
| Tenor sax | | 0.15 (0.15, 0.20) | 0.32 (0.05, 1.81) |
| Alto sax | | | 0.25 (0.16, 0.48) |
| Soprano sax | | | 0.44 (0.10, 3.01) |
| Clarinet | 0.24 | 0.56 (0.50, 1.21) | 0.35 (0.10, 28.0) |
| Bassoon | 0.04 | 0.21 (0.07, 0.35) | |
| Oboe | 0.50 | 2.27 (1.53, 3.94) | |
| Practice Chanter | | | 3.63* (1.32, 6.49) |
| G. H. Bagpipes | | | 0.98* (0.81, 1.09) |
| Sc. Smallpipes | | | 0.11* (0.08, 0.15) |
| C flute | 0.05 | 0.02 | 0.22 (0.045, 3.68) |
| Alto recorder | | | 0.58* (0.19, 1.08) |
| Fife | | | 0.06* (0.007, 0.23) |
| Piccolo | 0.046 | | 0.026* (0.006, 0.18) |
| Bb tuba | 0.02 | 0.25 | 0.18 (0.06, 0.41) |
| F tuba | | | 1.41* (0.90, 2.33) |
| Euphonium | | 0.59 | |
| French horn | 0.11 | 0.30 (0.04, 1.07) | 0.32* (0.17, 0.86) |
| Bass trombone | 0.47 | | |
| Tenor horn | | | 0.59 (0.18, 1.64) |
| Tenor trombone | | 0.53 (0.24, 0.73) | 3.27 (0.15, 12.3) |
| Trumpet | 3.13 | 0.95 (0.55, 1.83) | 0.80 (0.08, 3.11) |
| Kuhlo horn | | | 0.91* (0.19, 2.91) |
| Hunting horn | | | 0.18* (0.11, 0.42) |
| Piccolo trumpet | | | 0.41* (0.32, 1.83) |

Table 3: Comparison of the emitted particle number concentration $N$ from wind instruments in this work with the literature. Together with the median values, the minimum and maximum are shown in parenthesis. The data from this study were restricted to 0.5 µm and larger particle diameter to match the range of the APS used in the two other studies, which were He et al. (2021) and Stockman et al. (2021). The instrument types are grouped from low to high register in single-reed woodwind, double-reed woodwind, edge-blown woodwind, and brass. Median values from this study marked with an asterisk indicate that this instrument type was played by only one subject.

### *2.7. Exhalation pressure and its role in particle emission*

Subject 31 performed breathing experiments where the subject was exhaling through a tube (different diameters for different experiments) with the aim of taking the same time for exhalation for all the different experiments. As the breathing resistance through a narrow tube is much higher compared to a wide tube, the air velocity and the pressure within the airways will be different. For the tube diameters of 4 mm to 6 mm, there was not much difference in both number and volume concentration in comparison to normal breathing. For the 3 mm tube, we find an increase of number concentration by a factor of 2.9, and an increase of volume concentration by a factor of 2.3, which is larger than the within-subject variability for breathing. The results from this experiment show that faster air at higher pressure tends to yield higher number and volume concentration. This is important to understand the pitch dependence for some instruments (e.g. Subsection 2.11) and it possibly explains the lower emitted particle number concentration from a single mouthpiece compared to the whole instrument.

### *2.8. Within-subject variability*

For some subject-instrument combinations where $\geq 10$ samples were available, we found that the within-subject variability of total particle concentration can be approximated well by a Gaussian distribution ($r^2 \geq 0.9$). This is consistent with the findings in Bagheri et al. (2021a) for breathing and singing. The ratios of standard deviation $\sigma$ and mean $\mu$ are shown in table 4 for both total number concentration and total volume concentration. The high $\sigma/\mu$ ratios need to be considered when interpreting the emission from the same subject for different notes or different pieces of music as observed differences might be attributed to the within-subject variability.

Table 4: Standard deviation to mean ratios of Gaussian fits of total particle number/volume concentration from measurements with $\geq 10$ samples as a measure of within-subject variability.

| Subject | Instrument | Played | #samples | $N$: $\sigma/\mu$ [%] | $V$: $\sigma/\mu$ [%] |
|---|---|---|---|---|---|
| S7 | trumpet | Medley | 5 | 10 | 39 |
| S17 | double horn | Sonata | 12 | 36 | 33 |
| S17 | trombone | Sonata | 12 | 63 | 90 |
| S31 | hunting horn | note Bb3 | 13 | 39 | 77 |
| S31 | trumpet | note Bb3 | 26 | 53 | 54 |

### *2.9. Between-subject variability for same instrument type and music*

From 2 subjects playing the trumpet (note Bb3) and 2 subjects playing the alto sax (note Db3), we could not find a significant difference in emitted particle volume concentration. At maximum, the emitted volume concentration differed by a factor of 1.2. In contrast to trumpet and alto sax, we saw a significant difference in the emitted volume concentration for the same note played by four clarinetists playing the note D3 (difference up to factor 8.5), and for three flutists playing the note C4 (difference of almost a factor of 21).

### 2.10. Particle emission versus loudness

For one subject playing the same piece of music on a tenor sax in pianissimo (pp), mezzo forte (mf) and fortissimo (ff), we found the same relationship as He et al. (2021) did for reed instruments with a simple tube design, i.e. a monotonic increase of emitted $N$ for higher loudness. Compared to the emitted particle volume concentration in pianissimo, the emitted volume concentration in mezzo forte was by a factor of 2.2 higher, and in fortissimo, the emitted volume concentration was a factor of 5.5 higher.

### 2.11. Pitch dependence

We examined three brass instruments played by two subjects (a Kuhlo horn, a Fürst Pless hunting horn without valves, and a piccolo trumpet) in terms of particle emission for playing notes of different pitch. While the maximum emission was observed during playing a piece of music (piccolo trumpet and Kuhlo horn data), there was a tendency in all three brass instruments towards higher emitted $N$ for higher pitch. The particle size distributions from the Kuhlo horn are shown in Fig. 9 top as a representative example of the brass instruments. Due to the limited number of subjects and samples we cannot conclude if this is a general feature. From the physics perspective, it would make sense as higher notes need faster air, and oftentimes faster air means also more pressure which comes along with higher particle emission (see Subsection 2.7). What we also saw was a higher emitted number concentration for playing the first subharmonic compared to the first two harmonics (see Fig. 9 top). It is possible that the higher particle emission originates from a larger amount of air needed to create the tone in comparison to the first and second harmonic. A similar trend towards more particle emission for higher notes was found for two clarinet players with the size distribution of one of them shown as an example in Fig. 9 bottom.

The pitch dependence was also investigated for a piccolo, a C flute and a fife. For the edge-blown woodwind instruments, the result was inconclusive. While the high register of the C flute yielded higher particle number concentration compared to the low register (no overblowing), we saw the opposite for the fife where the emitted particle concentration became less for higher pitch. The piccolo had most particles emitted from the end piece if all tone holes were closed, but there was no observable trend for the other notes. Similar to what we saw for the piccolo or fife, the emitted particle concentration while playing a straight soprano sax in the low register was higher than in the high register.

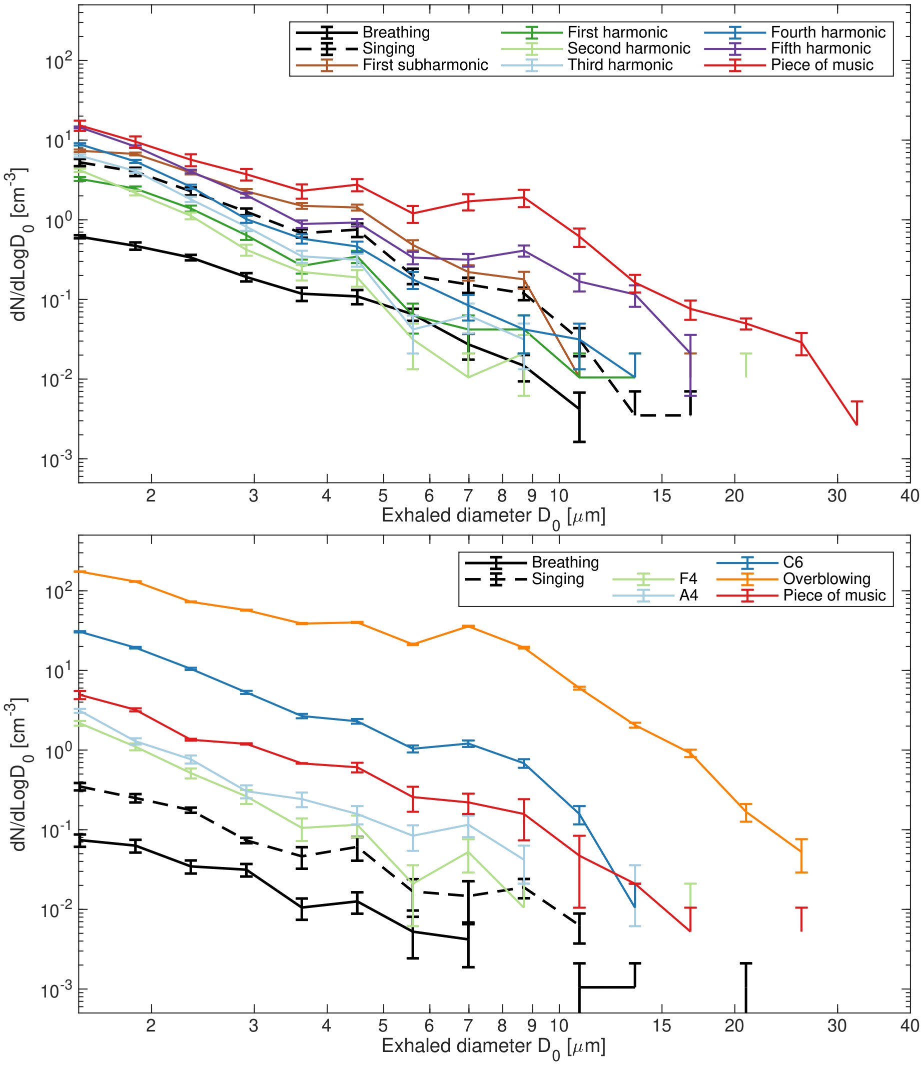


Figure 9: Particle size distributions for playing a Kuhlo horn (top) and a clarinet (bottom) for long notes at different pitch in comparison to breathing, singing and playing a piece of music. Shown are the first subharmonic (brown), first and second harmonic (green), third and fourth harmonic (blue), fifth harmonic (purple) and the piece of music (red) for the Kuhlo horn (top figure), and the notes F4 (green), A4 (light blue), C6 (dark blue), overblowing the reed (orange) and the piece of music (red) for the clarinet (bottom figure). The subject-specific median for breathing (solid black lines) and singing (dashed black lines) are shown as well.

### *2.12. Emission of particles* >6 µm *from brass mouthpieces*

In addition to the sizes below 10 µm measured by the OPS, we measured larger exhaled particles with the holography system. An example of data obtained from one hologram where the subject played a trumpet mouthpiece into the sample volume is shown in Fig. 10. This is a typical example of droplets primarily produced by the lip vibrations which would then enter the resonator tube of the brass instrument. Their median size is 12.5 µm (first quartile: $D_0 =$ 8.8 µm, third quartile: $D_0 =$ 20.6 µm), and the size distribution is approximately log-normal (see the red line in Fig. 10). In this case, the droplet number concentration $N$ was 1.1 cm$^{-3}$.

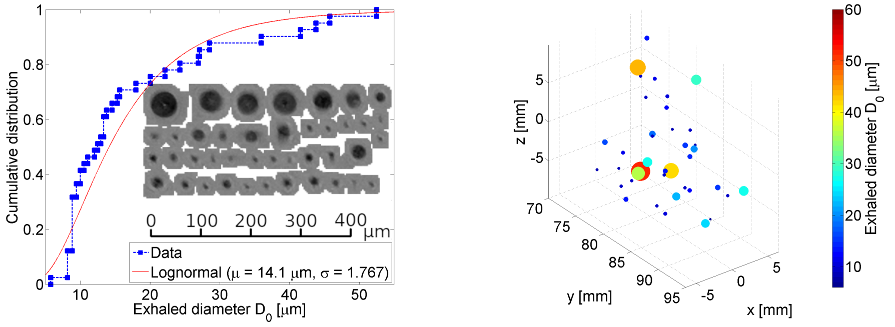


Figure 10: Example data from the holography setup where a trumpet mouthpiece was played. Shown are the cumulative size distribution and its log-normal approximation along with grayscale images of the particles (left), and the spatial distribution and size of the particles (color-coded and indicated by the marker size) in the center of the sample volume (right). The coordinates are streamwise away from the subject (x), crosswise to the right (y), and vertically upwards (z). The center of the sample volume is at $(x, y, z) = (0, 83, 0)$

### *2.13. Penetration of fabrics used for pandemic masks for wind instruments*

We tested the penetration of dry dolomite dust on five different melt-blown fabrics from different manufacturers, which were used as pandemic masks for the wind instruments. Into all of these materials, an electric charge was introduced during the manufacturing process. filter01 was classified as a F9 filter (equivalent ISO ePM1 80%), filter02 was classified as a F7 filter (equivalent ISO ePM1 50%), filter03 was a single layer melt-blown fabric with a density of 55 g m$^{-2}$, filter04 was a single layer melt-blown fabric with a density of 25 g m$^{-2}$, and filter05 was classified as a F8 filter (equivalent ISO ePM1 70%) but with special requirements for usage in dental laboratories (to filter out highly toxic dust containing cadmium or other heavy metals). The special requirement for filter05 might be the reason for having the lowest penetration of all the filters tested with dolomite dust (see Fig. 11, the experimental setup for testing the filters was the same as for testing the mask fabric penetration in Bagheri et al. (2021b)) with an average flow rate of 8.3 cm s$^{-1}$ (OPS only). The measured penetration for the thin fabrics was higher than for the thicker fabrics (the two thin

single-layer fabrics filter03 and filter04 had the highest penetration of all charged melt-blown materials tested). When examining the specific penetration $P(D)$ as a function of particle diameter more closely, we recognized that the mean value from the various penetration measurements for the same material can be fitted well with a power law. The two fit parameters are the penetration $P_1$ at 1 µm particle diameter, and the exponent $\beta$.

The relationship in Eq. 1 makes it very convenient for calculating the number of infectious units per unit time which could penetrate the mask. Fig. 11 shows the penetration of five filters used in the experiments. The values of $P_1$ and $\beta$ are shown in the upper right corner of Fig. 11.

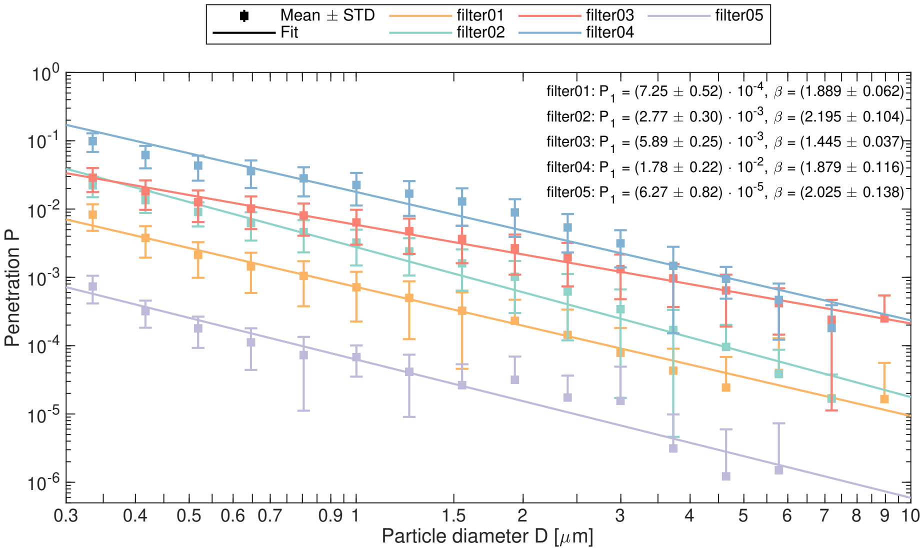


Figure 11: Measured penetration for filter01 (orange), filter02 (green), filter03 (red), filter04 (blue) and filter05 (purple) used in the experiments. Shown are mean penetration (squares) and standard deviation (errorbars). The solid line shows the power law fit with parameters given in the upper right corner.

$$P(D) = P_1 \cdot (D/1\,\mu\text{m})^{-\beta} \tag{1}$$

$$P(D) = P_0 \cdot \exp\left(-\beta \cdot (D/1\,\mu\text{m})\right) \tag{2}$$

In addition to the fabrics tested on the wind instruments, we received more samples. Their penetration was also measured. One of these fabrics (filter06) was a thick pink cloth that showed a similar dependence of penetration with particle size as a thin non-charged polypropylene fabric (filter10). Instead of a power law, we found an exponential decay to fit the measured penetration well (Eq. 2). When using a double layer of this material, the functional dependence did not change. We think that the static charge makes the difference in the

functional behavior. The penetration for both kinds of fabric is shown in Fig. 12. Two more F9 filters (filter07 and filter08) were tested as well and behaved similar to filter01 in Fig. 11. A multi-layer polypropylene fabric with static charge (filter11) behaves as the fabrics tested before (power law dependence). Another sample of multi-layer melt-blown mask fabric (which is filter12), together with filter 11, show similar penetration as the F9 filters.

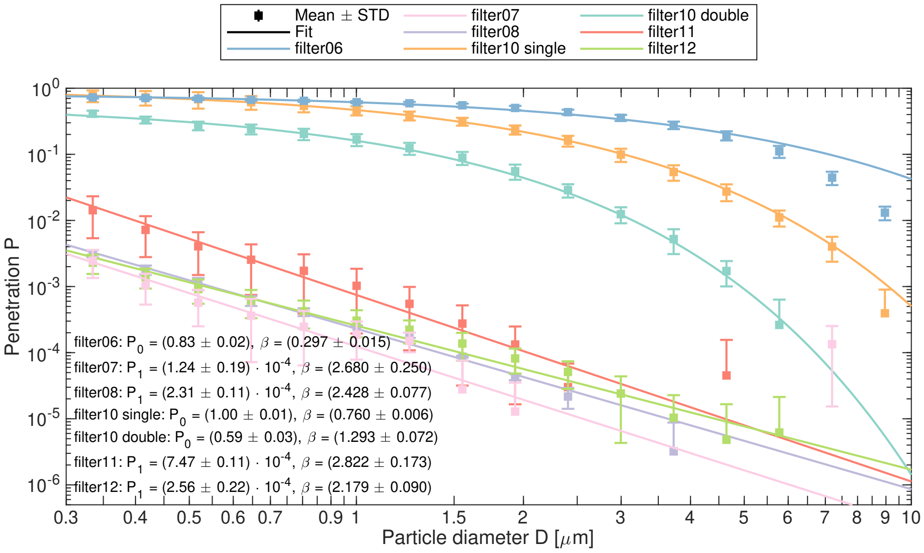


Figure 12: As in Fig. 11 for filter06 (blue), filter07 (pink), filter08 (purple), filter10 single layer (orange), filter10 double layer (dark green), filter11 (red), and filter12 (light green). The solid lines show the power law fit (filters 07,08,11 and 12) or the exponential fit (filters 06 and 10) with parameters given in the lower left corner. The two outliers for filter11 (at 4.5 µm) and filter07 (at 7 µm) were ignored for the fit.

## *2.14. The filter fabric as a particle source*

In order to investigate the possibility of systematic errors during the measurement on the instrument masks, we put a sample of filter05 (a brand new sample which was unpacked in the MPIDS cleanroom) over the 100 mm sampling funnel and connected the OPS. In the first experiment, cleanroom air was being sucked through the filter, where just one particle of 0.34 µm diameter could be detected. Also, we tipped the funnel for 1 min with the finger to ensure that there are no particles being produced from the funnel itself or from somewhere in the tubing. This test did not show any particle count. Finally, we tipped the filter fabric with the finger and measured the particle concentration for 2 min. In this test, we found a flat size distribution across the entire sampling range of the OPS (see Fig. 13). This finding means that there must be particles either captured within the fabric, or fibers detaching from the fabric if repeated mechanical stress is exercised on the filter fabric. Particles emitted

from a brand new filter sample need to be taken into account when examining the performance of a filter in a measurement on the wind instrument. Any flat size distribution with some large (above 1 µm) particles is suspicious, so that the general recommendation is to do a plausibility check first. If there are particles detected in the measurement, which are more than one order of magnitude more abundant than expected from the theoretical penetration, these particles are most likely artifacts and should not be used to calculate particle volume concentration when discussing the infection risk.

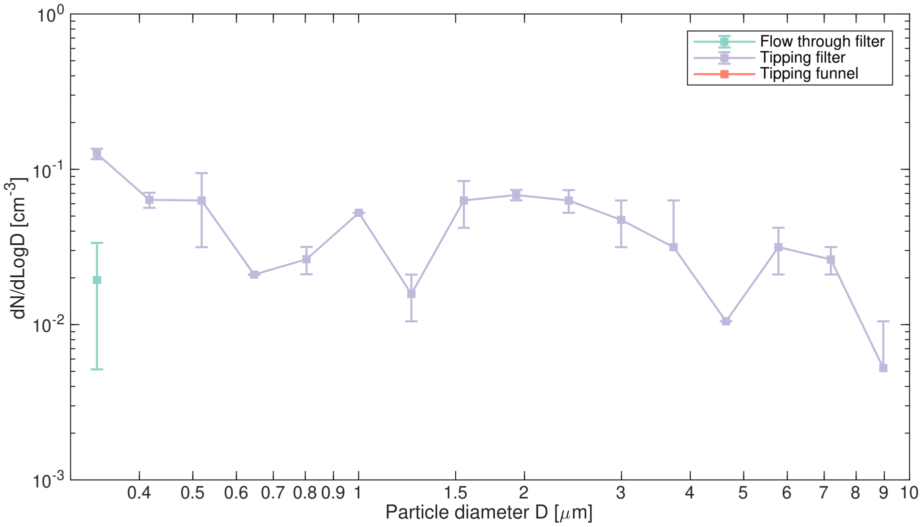


Figure 13: Measured size distributions from an experiment with cleanroom air going through the filter (green), tipping the filter (purple) and tipping the funnel (red).

### *2.15. Comparison of the measured filter penetration with conditions during playing music*

The filter penetration was measured with a filter holder which had a 16 mm circular aperture. Depending on the experimental setup, the volume sampling rate was either $1.75\,\mathrm{L\,min^{-1}}$ (with SMPS) or $1.00\,\mathrm{L\,min^{-1}}$ (OPS only). From the aperture diameter and the volume sampling rate, the average air velocity through the fabric can be calculated. With SMPS and OPS, we had $v = 14.5\,\mathrm{cm\,s^{-1}}$, with OPS only we had $v = 8.3\,\mathrm{cm\,s^{-1}}$. We know that the penetration of a filter fabric is velocity-dependent. As the brass instruments have typical bell diameters, the maximum exhalation volume flux for each configuration can be computed. This is the upper bound at which the measured penetration is still valid. If we take the smallest bell of the brass family, which is the piccolo trumpet, we obtain a volume flux of $39\,\mathrm{L\,min^{-1}}$ to reach a mean velocity of $v = 8.3\,\mathrm{cm\,s^{-1}}$. The peak exhale rate found by Bouhuys (1964) for the trumpet was $0.469\,\mathrm{L\,s^{-1}}$, which yields an upper bound of $28.1\,\mathrm{L\,min^{-1}}$ for the

exhale rate while playing trumpet. Due to the larger bell diameter, it is obvious that the low brass instruments will never reach such high velocities. Thus, our measured penetration at $v$ =8.3 cm s$^{-1}$ can be used as an absolute upper bound for the expected penetration while the filter is attached to a brass instrument which is being played. This means that something must have gone wrong if the measured particle size distribution from playing brass with filter is higher than the size distribution without filter multiplied by the penetration (which is the theoretical size distribution from playing brass with filter). However, as described in Subsection 2.14, the filter fabric itself can release particles, which is most obvious to see in the larger sizes. More details are discussed in Subsection 2.16.

### *2.16. Measured versus expected filter penetration*

With one filter fabric (here: filter02) we present two typical scenarios observed in the test. The first subject used this filter on a trumpet and the filter was only used in the MPI-DS cleanroom with the measured size distributions shown in Fig. 14 top. The other subject used the filter on a trombone in different occasions outside the cleanroom before the measurement. We placed the funnel directly on the mask to avoid dilution or bypass flow of cleanroom air. As already mentioned in Subsection 2.14, touching the filter with the funnel and possibly moving the funnel around on the filter surface is known to create particles which come from the fabric itself. While the penetration of the particles smaller than 1.5 µm dry diameter is as expected, there are also particle counts in the larger bins, well above the expected penetration in case of the trombone player (see Fig. 14 bottom). On the trumpet, there was only one particle count at 2 µm diameter which is suspicious. We interpret the large particles in case of the trombone as artifacts from either detaching fiber fragments or dust on the outer layer of the filter (this was the filter that has been used outside the cleanroom). The fact that some particle sizes were only found in the play with filter, but not in the unfiltered case, strengthens this argument.

When discussing mask efficacy and infection risk, it makes sense to use the expected penetration for the dry particle diameter (the blue lines in Fig. 14). In two additional experiments where we used filter05 on two trumpets, we found two particles each, penetrating the filter. Due to the very limited counting statistics and the reasonable agreement between the calculated penetration for dry particle diameter in Fig. 14, we decided to use the dry expected penetration for the calculation of the upper bound of infection risk.

In contrast to the penetration following the blue or red curve (Fig. 14), the mask material filter05 with penetration shown in Fig. 15 is very efficient in capturing particles. In Fig. 15 top, only one particle penetrated the fabric, and in Fig. 15 bottom, there were two particles total that passed the fabric. Materials with such low penetration of particles between 0.3 and 10 µm dry diameter need to be examined either with test aerosol or the duration of playing needs to be very long to yield penetration data above the noise floor.

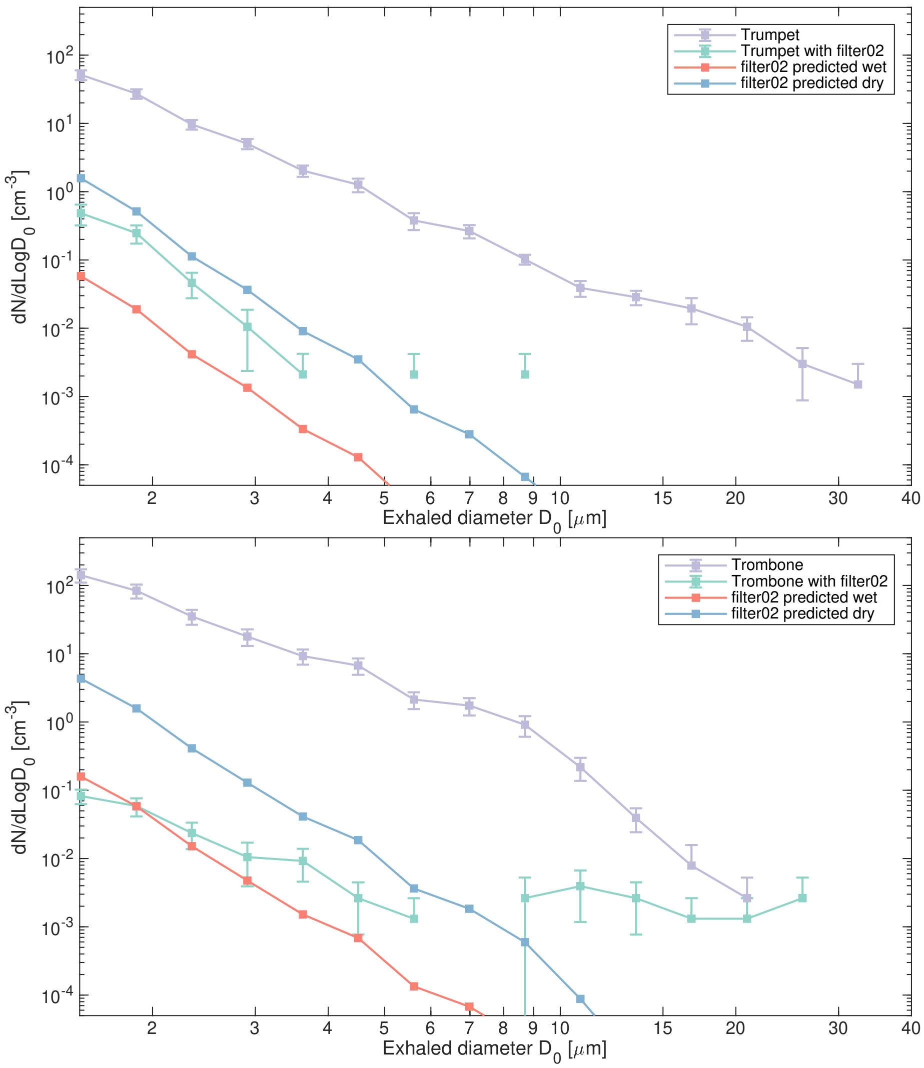


Figure 14: Particle size distribution from playing the trumpet (top figure) as usual (purple) and from using filter02 as a mask (green). Shown are also the expected size distribution based on penetration measurements of the filter fabric and the power law fits under the assumption of dry particles entering the filter (blue) or wet particles entering the filter (red). Errorbars represent the larger uncertainty from either counting statistics or standard error. The second example (bottom figure) is for playing the trombone.

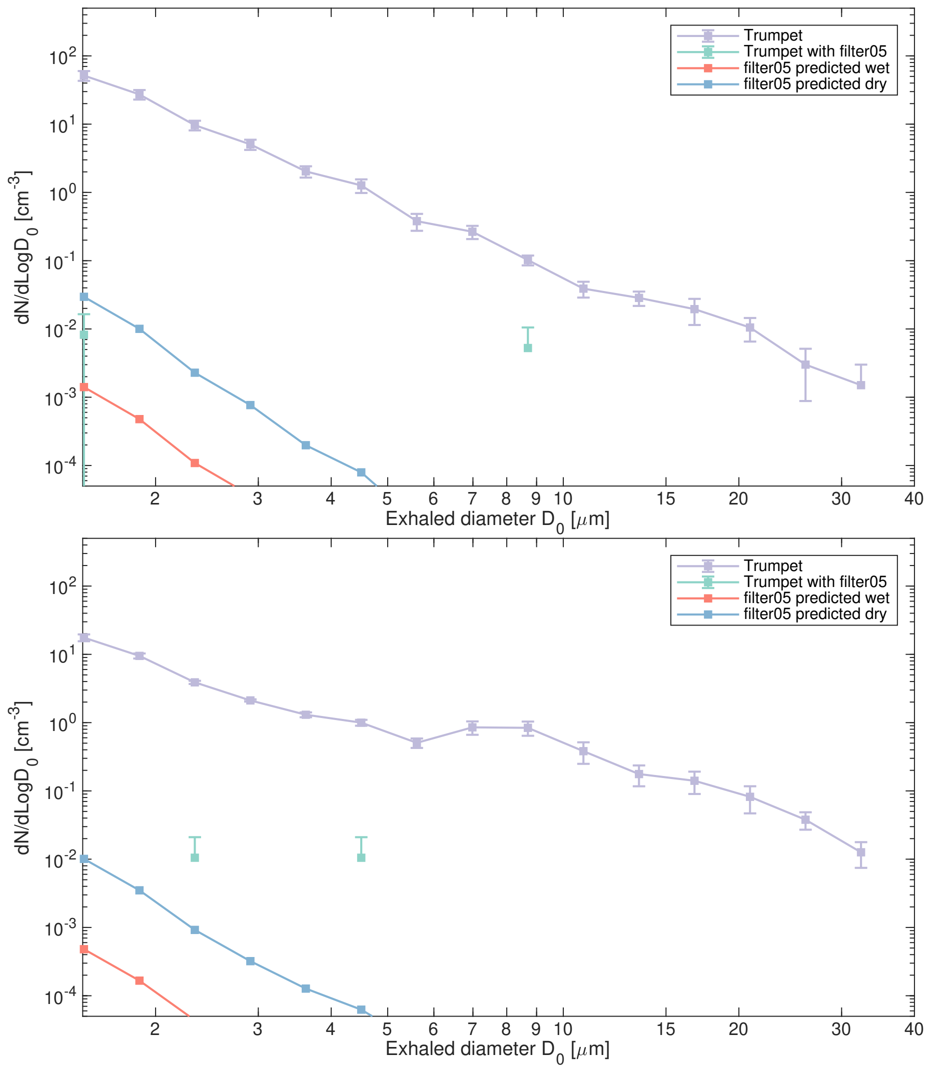


Figure 15: As in Fig. 14 for filter05 tested by two trumpet players on two different trumpets.

### *2.17. The effect of the SARS-CoV-2 variant on infection risk in the near-field*

Besides the original strain of SARS-CoV-2, several other strains have been circulated in the meantime. While the original strain is thought to have a typical value of the 63.21% infectious dose $ID_{63}$ around 400 - 450 with a range from 100 to 1000 (Nordsiek et al., 2021), based on the data for SARS-CoV-1 in Watanabe et al. (2010), the other strains relevant for most European countries and also for the U.S. are B.1.617.2 (Delta) with $ID_{63} = 200$, and, most recently, B.1.1.529 (Omicron) with $ID_{63} = 70$. Here, we need to mention that all these values of $ID_{63}$ have a range of uncertainty of a factor 3.2 based on the discussion in Nordsiek et al. (2021). The calculations of $ID_{63}$ for Delta and Omicron are based on the value for the original strain (which is also called "wild type") and the results of the study by Chen et al. (2021) who compared the binding energy of the receptor binding domain at the spike of the virus for the Delta and Omicron variant against the original strain. Omicron is about 2.8 times more infectious than Delta (Chen et al., 2021). From Eq. 1 in the main paper, it is obvious that a change in $ID_{63}$ has the same effect on the risk of SARS-CoV-2 transmission as a change in $\mu$, which could be caused by lower or higher $\rho_p$. Based on the values of $ID_{63}$ summarized in this subsection, we show the effect of higher infectivity on the infection risk for the near-field scenario without masks but with 1.5 m distance in Fig. 16. Qualitatively, the other exposure scenarios will look very similar. Despite the uncertainties in the exact values of $ID_{63}$, the relationship between the different strains in terms of infection risk will be quite accurate. In addition to the usage of masks, testing can also help to reduce the transmission risk by limiting $\rho_p$ to $<10^6$ cm$^{-3}$ for a rapid diagnostic test with good sensitivity and correct sampling. The dashed lines in Fig. 16 indicate how regular testing can help to mitigate the risk of SARS-CoV-2 transmission even further.

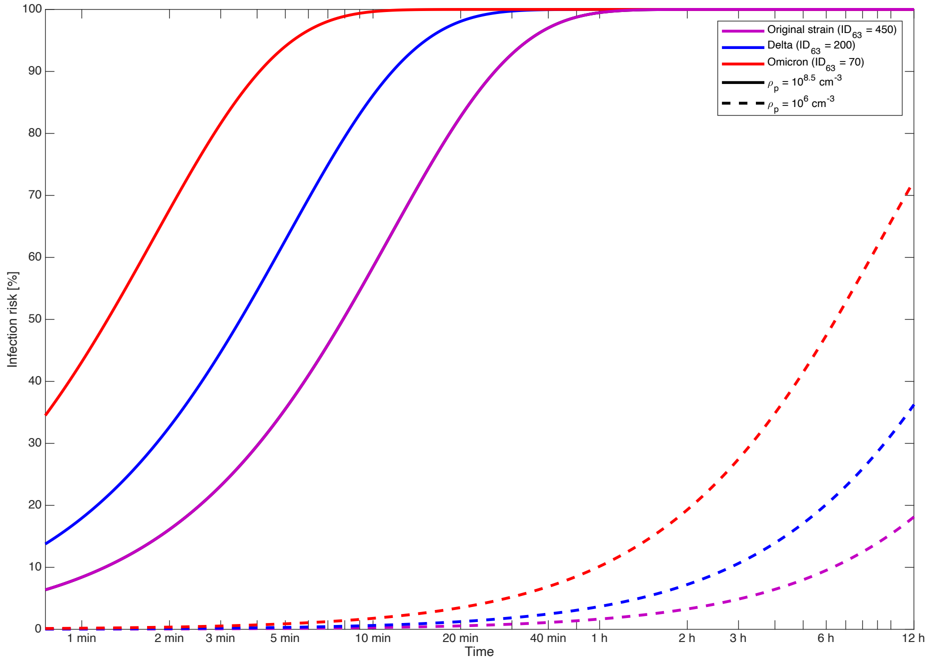


Figure 16: Risk of SARS-CoV-2 transmission (abbreviated "infection risk") as a function of time as in Fig. 5 of the main paper for the high emission instrument and the "Distancing" exposure scenario with different strains of SARS-CoV-2 leading to different values of $ID_{63}$ (color-coded). The solid lines indicate typical pathogen concentration for highly infectious individuals, the dashed lines indicate infectious individuals carrying SARS-CoV-2 despite being tested negative via antigen rapid diagnostic test. The distance between susceptible and infectious is 1.5 m, no masks are used here.

## 2.18. The effect of different instrument-mask materials

As already discussed in Subsection 2.13, the different mask materials which were tested had different penetration as a function of particle diameter. With the near-field and far-field model, it has been investigated how much the usage of a different mask material affects the risk of airborne SARS-CoV-2 transmission. In addition to our best material (filter05), we chose the thinnest uncharged material (filter10) and one of the thinnest charged materials (filter03) to compete against filter05. As shown in Fig. 17, there is no visible difference between filter03 and filter05 for the low-emission instrument, and the infection risk upon exposure to a low-emitter with filter10 is about the same as for a high-emitter with filter03. Even more interesting is the comparison of the different mask materials in the far-field model with 4 ACH. The solid lines in Fig. 18 show the "Room-Unmasked" scenario for comparison. Here, a visible difference is found between "Room-Instrument-mask (filter10)" and "Room-Instrument-mask (filter03)" for the high emission instrument. But the difference between the infection risk with filter03 compared to filter05 is marginal for both high-emitter and low-emitter. For the low-emitter, there is even no visible difference between "Room-Instrument-mask (filter10)" and the other mask materials.

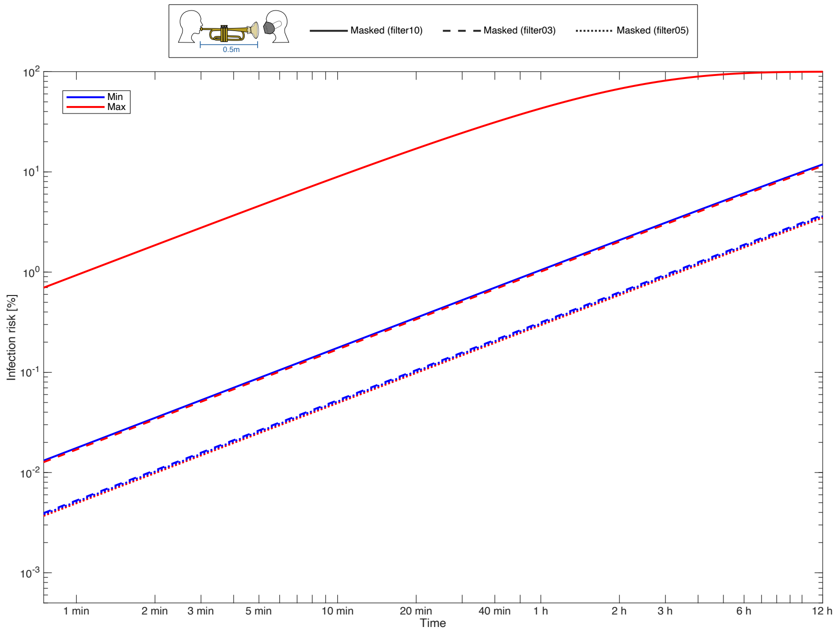


Figure 17: Infection risk for near-field exposure scenario "Masked" as a function of time. Shown are infection risk as a function of time for high-emitter (red) and low-emitter (blue) instrument for an instrument-mask made of filter10 (solid lines), filter03 (dashed lines), and filter05 (dotted lines).

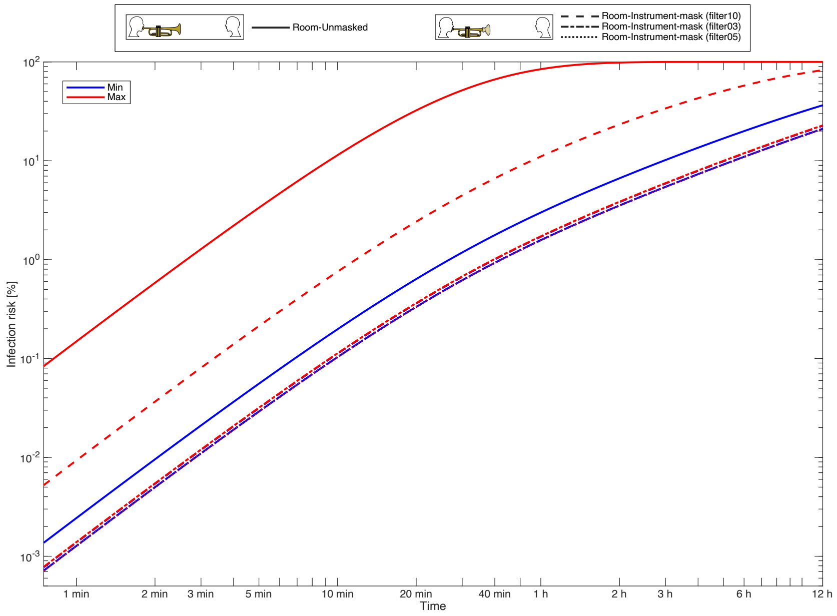


Figure 18: As in Fig. 17 for the far-field exposure scenario. Shown are the scenarios "Room-Unmasked" (solid lines), "Room-Instrument-mask (filter10)" (dashed lines), "Room-Instrument-mask (filter03)" (dash-dotted lines), and "Room-Instrument-mask (filter05)" (dotted lines).

## References


Bagheri, G., Schlenczek, O., Turco, L., Thiede, B., Stieger, K., Kosub, J.M., Pöhlker, M., Pöhlker, C., Molacek, J., Scheithauer, S., Bodenschatz, E., 2021a. Exhaled particles from nanometre to millimetre and their origin in the human respiratory tract. medRxiv preprint URL: https://doi.org/10.1101/2021.10.01.21264333, doi:10.1101/2021.10.01.21264333. version 1, 03 Oct 2021.

Bagheri, G., Thiede, B., Hejazi, B., Schlenczek, O., Bodenschatz, E., 2021b. An upper bound on one-to-one exposure to infectious human respiratory particles. Proceedings of the National Academy of Sciences 118. URL: https://www.pnas.org/content/118/49/e2110117118, doi:10.1073/pnas.2110117118.

Bouhuys, A., 1964. Lung volumes and breathing patterns in wind-instrument players. Journal of Applied Physiology 19, 967–975. URL: https://doi.org/10.1152/jappl.1964.19.5.967, doi:10.1152/jappl.1964.19.5.967. PMID: 14207753.

Chen, J., Wang, R., Gilby, N.B., Wei, G.W., 2021. Omicron (B.1.1.529): Infectivity, vaccine breakthrough, and antibody resistance. arXiv preprint doi:10.48550/arXiv.2112.01318, arXiv:2112.01318. version 1, 01 Dec 2021.

Firle, C., Steinmetz, A., Stier, O., Stengel, D., Ekkernkamp, A., 2021. Aerosol emission rates from playing wind instruments - implications for covid-19 transmission during music performance. medRxiv preprint URL: https://www.medrxiv.org/content/early/2021/12/11/2021.12.08.21267466, doi:10.1101/2021.12.08.21267466. version 1, 11 Dec 2021.

He, R., Gao, L., Trifonov, M., Hong, J., 2021. Aerosol generation from different wind instruments. Journal of Aerosol Science 151, 105669. URL: https://www.sciencedirect.com/science/article/pii/S0021850220301555, doi:10.1016/j.jaerosci.2020.105669.

Nordsiek, F., Bodenschatz, E., Bagheri, G., 2021. Risk assessment for airborne disease transmission by poly-pathogen aerosols. PLoS ONE 16, 1–41. doi:10.1371/journal.pone.0248004.

Pöhlker, M.L., Krüger, O.O., Förster, J.D., Berkemeier, T., Elbert, W., Fröhlich-Nowoisky, J., Pöschl, U., Pöhlker, C., Bagheri, G., Bodenschatz, E., Huffman, J.A., Scheithauer, S., Mikhailov, E., 2021. Respiratory aerosols and droplets in the transmission of infectious diseases. arXiv preprint doi:10.48550/arXiv.2103.01188, arXiv:2103.01188. version 4, 04 Aug 2021.

Stockman, T., Zhu, S., Kumar, A., Wang, L., Patel, S., Weaver, J., Spede, M., Milton, D.K., Hertzberg, J., Toohey, D., Vance, M., Srebric, J., Miller, S.L., 2021. Measurements and Simulations of Aerosol Released while Singing and

Playing Wind Instruments. ACS Environmental Au 1, 71–84. URL: https://doi.org/10.1021/acsenvironau.1c00007, doi:10.1021/acsenvironau.1c00007.

Watanabe, T., Bartrand, T.A., Weir, M.H., Omura, T., Haas, C.N., 2010. Development of a Dose-Response Model for SARS Coronavirus. Risk Analysis 30, 1129–1138. URL: https://onlinelibrary.wiley.com/doi/abs/10.1111/j.1539-6924.2010.01427.x, doi:https://doi.org/10.1111/j.1539-6924.2010.01427.x.

von der Weiden, S.L., Drewnick, F., Borrmann, S., 2009. Particle Loss Calculator – a new software tool for the assessment of the performance of aerosol inlet systems. Atmospheric Measurement Techniques 2, 479–494. URL: https://amt.copernicus.org/articles/2/479/2009/, doi:10.5194/amt-2-479-2009.
